# Supplementary material for: Synthetic photonic lattices: new routes towards all-optical photonic devices
Source: arXiv:1612.08467 source file (2016-12-27)
Supplement: Supplementary file 1 [file Luo_supp-09-28.pdf]

# Supplementary Materials

Xi-Wang Luo,[1,2] Xingxiang Zhou,[1,2,*] Jin-Shi Xu,[1,2] Chuan-Feng Li,[1,2] Guang-Can Guo,[1,2] Chuanwei Zhang,[3] and Zheng-Wei Zhou[1,2,†]

[1]*Key Laboratory of Quantum Information, University of Science and Technology of China, Hefei, Anhui 230026, China*
[2]*Synergetic Innovation Center of Quantum Information and Quantum Physics, University of Science and Technology of China, Hefei, Anhui 230026, China*
[3]*Department of Physics, The University of Texas at Dallas, Richardson, Texas 75080, USA*

## I. EFFICIENCY FOR ABSORPTION AND EMISSION OF THE PHOTON SIGNAL

The photon signal to be stored has a finite bandwidth around a peak frequency $\omega_0$, which matches the resonant frequency of the main cavity. When the signal enters the cavity, the occupied central Bloch momentum is determined by solving

$$2\kappa\cos(K-\phi)=0. \tag{1}$$

$\phi=0$ during the write-in process, yielding $K_\alpha=\pi/2$ and $K_\beta=-\pi/2$. Consequently, two pulses with Bloch momenta $K_\alpha$ and $K_\beta$ start to propagate in the OAM lattice with opposite group velocities

$$v_g=\frac{\partial\omega}{\partial K}|_{K=\pm\frac{\pi}{2}}=\pm 2\kappa. \tag{2}$$

The read-out process, during which $\phi$ is set to $\pi$, is the time reversal to write-in. The velocities of the signal in the OAM lattice are reversed and the signal propagates back to the $l=0$ mode as shown in Fig. 4 (a) in the main text.

We analyze the read-out efficiency assuming that the only loss of the cavity modes is due to coupling to the input and output fields, i.e. $\gamma_j=\delta_{j,0}\bar{\gamma}$ with the coupling rate $\bar{\gamma}=\frac{1-\sqrt{R_\mathrm{h}}}{\pi\sqrt[4]{R_\mathrm{h}}}\Omega_0$ [1] determined by the intensity reflectivity $R_\mathrm{h}$ of the input/output pinhole and the free spectral range (FSR) $\Omega_0$ of the cavity. Since only $l=0$ mode is coupled with the input and output fields, the cavity field equation (in Heisenberg picture) is

$$\begin{aligned}\frac{d}{dt}a_j(t) &= -i\omega_0+i\kappa[e^{i\phi}a_{j+1}(t)+e^{-i\phi}a_{j-1}(t)]\\ &\quad -\frac{\gamma_j}{2}a_j(t)+\delta_{j,0}\sqrt{\bar{\gamma}}\hat{E}^0_\mathrm{in}(t).\end{aligned} \tag{3}$$

For a quantum single-photon pulse, the state of the system (in Schrödinger picture) is $|\Psi(t)\rangle=\sum_j\alpha_j(t)|1_j\rangle+\int d\omega\widetilde{E}^0(\omega,t)|1_\omega\rangle$, with $|1_j\rangle=a_j^\dagger|0\rangle$ being the state of a single photon occupying the $j$-th mode, and $|1_\omega\rangle=b_\omega^\dagger|0\rangle$ being the single photon state in the input/output channel with frequency $\omega$. Initially $\alpha_j(t_0)=0$ ($t_0\to-\infty$) for all $j$. The coefficients $\alpha_j$ obey same dynamics as Eq. 3 with $a_j$ replaced by $\alpha_j(t)$, and the input field operator replaced by the temporal input-pulse $E^0_\mathrm{in}(t)=\frac{1}{\sqrt{2\pi}}\int d\omega\widetilde{E}^0(\omega,t_0)e^{-i\omega(t-t_0)}$. The temporal output-pulse, $E^0_\mathrm{out}(t)=\frac{-1}{\sqrt{2\pi}}\int d\omega\widetilde{E}^0(\omega,t_1)e^{-i\omega(t-t_1)}$ with $t_1\to+\infty$, can be obtained as $E^0_\mathrm{out}(t)=\sqrt{\bar{\gamma}}\alpha_0(t)-E^0_\mathrm{in}(t)$ [2].

For a classical coherent state pulse, the state of the system (in Schrödinger picture) now becomes $|\Psi(t)\rangle=\bigotimes_j|\alpha_j(t)\rangle\otimes|\mathcal{E}(t)\rangle$, where $|\alpha_j(t)\rangle$ is the coherent state of the $j$-th mode satisfying $a|\alpha_j(t)\rangle=\alpha_j(t)|\alpha_j(t)\rangle$, and $|\mathcal{E}(t)\rangle$ is the classical coherent photon state in the input/output channel, satisfying $b_\omega|\mathcal{E}(t)\rangle=\widetilde{E}^0(\omega,t)|\mathcal{E}(t)\rangle$. The coefficients $\alpha_j(t)$ and $\widetilde{E}^0(\omega,t)$ obey the same dynamics and same input/output relation as that for the single photon pulse because the dynamics of our system is characterized by the linear equation of photon operators (see Eq. 3).

The condition $E^0_\mathrm{in}(t)=0$ during the read-out leads to $E_\mathrm{out}(t)=\sqrt{\bar{\gamma}}\alpha_0(t)$. In a short time interval $[t,t+dt]$ during the read-out, the number of photons emitted from the $l=0$ cavity mode into the output field is $\Delta N_1=|E^0_\mathrm{out}(t)|^2dt=\bar{\gamma}|\alpha_0(t)|^2dt$. Meanwhile, the number of photons in the cavity that propagate from $l\neq0$ modes back to the $l=0$ mode is $\Delta N_2=2|v_g||\alpha_0(t)|^2dt$. When

$$\bar{\gamma}=2|v_g|, \tag{4}$$

we have $\Delta N_1=\Delta N_2$, implying that the signal is read out with an efficiency of 100% [3]. Similar analysis applies to the write-in process. This conclusion is confirmed by the simulation results in Fig. 4 (a) in the main text which are obtained by numerically solving Eq. (3).

## II. PHOTON LOSS

Imperfections such as photon loss will degrade the performance of the quantum memory and limit its storage time. There are 4 major sources of photon loss in our system due to:

- Finite finesse of the cavity;
- Absorption by the phase modulator;
- Limited efficiency of the SLMs;

*email: xizhou@ustc.edu.cn
†email: zwzhou@ustc.edu.cn

- Leakage through the input/output pinhole.

In the following, we analyze each loss mechanism and evaluate the overall effect of the photon loss on the performance of the quantum memory.

Intrinsic loss due to the finite finesse of the cavity can be very low as long as high quality cavities are used. Experimentally, finesse as high as $\mathcal{F} = 10^5$ has been demonstrated in ring-type optical cavities [4]. For a free spectral range $\Omega_0 \approx 1$ GHz, the corresponding intrinsic cavity loss $\gamma^{\mathcal{F}} \equiv \frac{\Omega_0}{\mathcal{F}}$ is on the order of 10 kHz. Much smaller than that from other sources, such loss is not expected to be the limiting factor for the storage time of the quantum memory.

The phase modulators introduce photon loss due to absorption by their optical media. With very low-loss material [5], such loss can be made lower than $10^{-3}$ for a medium thickness sufficient to generate a phase shift of $\pi$ required in our control protocol. The SLMs used to increase/decrease the OAM number introduce photon loss too because of their limited resolution and fabrication error. Such loss can be made very low as the efficiency of the SLMs can be very close to 100% with appropriate design and experimental techniques [6–8]. The effect of the phase modulator and SLM loss is further reduced by the fact that the auxiliary cavity is designed with destructive interference with very little photon signal. The effective photon loss for the main cavity field caused by the phase modulators and SLMs can be characterized by an overall decay rate [1]

$$\gamma^{\mathrm{A}} \simeq \frac{|r_B|^2}{2} \cdot \Omega_0 \frac{2(1-\sqrt{\eta^{\mathrm{A}}})}{\pi} = 4 \times (1-\sqrt{\eta^{\mathrm{A}}})\kappa, \quad (5)$$

where $r_B$ is the reflectivity of the coupling beam splitter and $\eta^{\mathrm{A}}$ is a parameter close to 1 determined by the phase modulator and SLM loss.

The rotationally symmetric input/output pinhole does not affect the OAM number of the cavity modes, though it may slightly modify the radial field distribution of low OAM modes. It can introduce photon loss in two ways. First, a small portion of the $l = 0$ input field falls outside of the pinhole and cannot enter the cavity regardless of the size of the pinhole since in theory the radius of the field distribution for a Gaussian pulse is infinite. Second, a small portion of the $l \neq 0$ modes in the cavity can leak out of the cavity via the pinhole. The leakage is more serious for low $l$ modes, and less severe for higher $l$ modes whose peak field distribution is farther away from the center. These loss channels cannot be overcome by simply increasing or decreasing the radius of the pinhole. Doing so will alleviate one mechanism but make the other worse. It is possible to improve both by using SLMs with a larger step index $M > 1$ and a pinhole large enough to couple in most of the Gaussian input field. The consequence of doing so is that the SLMs change the OAM number of the passing light beam by $\Delta l = M > 1$, and the OAM states that the signal propagate to become $jM$ with $j$ any integer. This smart technique to minimize

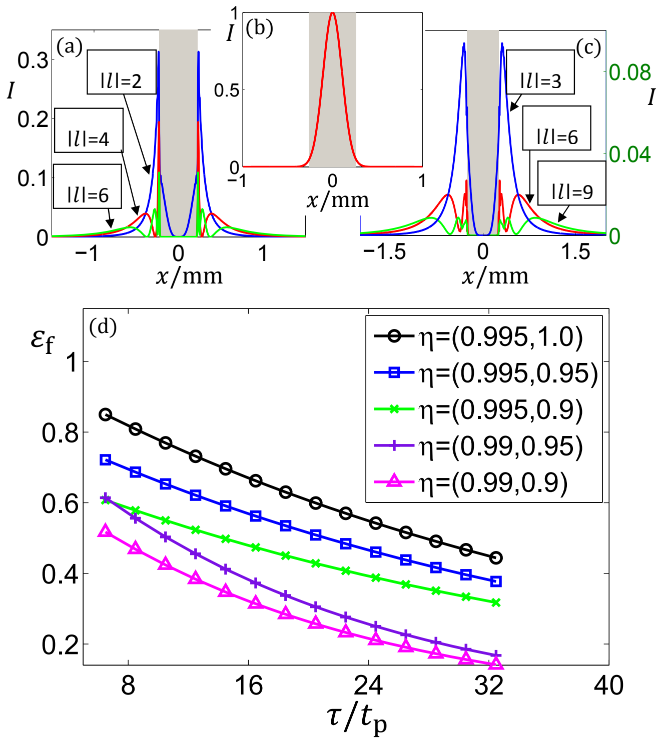


Figure S1: Dependence of photon loss on the step index $M$ of the SLMs and its effect on the storage efficiency of the quantum memory. The cavity mirrors' focal length, the wavelength of the optical signal, and the width of the signal's beam waist, are 7.5cm, 880nm, and 0.12mm, respectively. The beam splitters and SLMs are assumed to be placed where the beam waist is located. (a) Transverse field distribution along the $x$-axis on the input/output mirror plane $x-y$, calculated using Collins integral [9] with a step index $M = 2$ for the SLMs. The gray area marks the low-reflectivity pinhole whose radius is 0.225mm. The resulting efficiency is $\eta^{\mathrm{hole}} \simeq 90\%$. (b) Transverse field distribution of the $l = 0$ mode, most of which falls within the pinhole. (c) The same as in (a), except that the step index of the SLM is $M = 3$, and the radius of the pinhole is 0.26mm. The efficiency is about 95%. (d) Calculated storage efficiency versus storage time $\tau$. The input pulse is $E^0_{\mathrm{in}} = \exp(-\frac{t^2}{2t_{\mathrm{p}}^2} - i\omega_0 t)$, with $t_{\mathrm{p}} = 2.5\kappa^{-1}$ and $\eta = (\eta^{\mathrm{A}}, \eta^{\mathrm{hole}})$.

losses caused by the pinhole has its own limitation and can only be leveraged to a certain extent. A larger step index $M$ requires finer resolution and better error control in the fabrication of the SLMs. Such challenges may reduce the efficiency of the SLMs. Since the step in the OAM numbers is larger, the maximum OAM state that the cavity needs to support increases too. In Figs. S1 (a), (b), and (c), the field intensity distributions of a few low OAM modes on the input/output mirror are shown for different $M$ for the SLMs. It can be seen that a higher $M$ together with an appropriate pinhole radius results in reduced photon loss.

Aside from its coupling to the input/output field, the $l = 0$ mode can also have additional leakage due to the coupling to $l \neq 0$ modes. The part of these modes that

falls in the pinhole can escape quickly at a rate determined by the pinhole's coupling efficiency, which manifests as an additional loss

$$\gamma_0^{\mathrm{hole}} \approx 2(1-\eta^{\mathrm{hole}})\kappa \tag{6}$$

for the $l = 0$ mode. Here $\eta^{\mathrm{hole}}$ is a coefficient close to 1 determined by the portion of the higher modes' intensity distribution that falls outside the pinhole. Loss rate $\gamma_j^{\mathrm{hole}}$ for mode $jM$ can be calculated similarly. It is expected that $\gamma_j^{\mathrm{hole}}$ decreases very quickly with $j$, since the leakage via the pinhole is much smaller for higher OAM modes.

Considering all major sources of loss discussed above, we have

$$\gamma_j = \gamma^{\mathcal{F}} + \gamma^{\mathrm{A}} + \delta_{0,j}4\kappa + \gamma_j^{\mathrm{hole}} \tag{7}$$

for the $j$-th used OAM mode. Different terms in Eq. (7) are not equally important in determining the storage time of the quantum memory. As discussed earlier, $\gamma^{\mathcal{F}}$ is much smaller than other loss rates. The effect of the leakage via the pinhole is also limited. During the read-in phase, the low OAM modes are populated and they have some small leakage. However, such leakage does not have a dramatic effect on the storage time as long as the loss rate of these low OAM modes is much smaller than the group velocity of the signal in the OAM space. This is because, as shown in Fig. 5 in the main text, before the main intensity of the signal pulse can be lost by leakage via the pinhole, it already travels to higher OAM modes whose leakage is much lower. In the storage phase, the signal is safely kept in high OAM modes where the leakage via the pinhole is very low.

With the state of current technologies, the remaining loss channels by the phase modulators and SLMs are then the limiting factors for the storage time of the quantum memory. Their effect is persisting, even during the storage phase when transitions between OAM modes by the two auxiliary cavities [see Fig. 5 (a) in the main text] cancel each other and the signal is frozen in the OAM lattice [see Fig. 5 (e) in the main text].

In calculating and plotting (see Fig. 5 in the main text) the evolution of the signal pulse in the OAM space by numerically solving Eq. (3), we assumed a relatively high loss rate $\gamma_0^{\mathrm{hole}} = 0.2\kappa$ for the $l = 0$ mode to get a conservative result. Since $\gamma_j^{\mathrm{hole}}$ decreases very quickly with $j$ and the pinhole leakage is not the limiting factor for the storage time, the specific dependence of $\gamma_j^{\mathrm{hole}}$ on $j$ has little effect on the results. We simply use an exponential decaying function $\gamma_j^{\mathrm{hole}} = \gamma_0^{\mathrm{hole}} e^{-|j|}$. In Fig. S1 (d), we plot the calculated storage efficiency $\varepsilon_{\mathrm{f}}$ for the quantum memory [10] as a function of the storage time $\tau$ under different values of $\eta^{\mathrm{A}}$ and $\eta^{\mathrm{hole}}$. It is seen that the overall efficiency of the phase modulators and SLMs, $\eta^{\mathrm{A}}$, has a substantial impact on the storage time. Appreciable improvement can be achieved by lowing the loss of the phase modulators and SLMs.

## III. ESTIMATION OF THE FILTERING SHAPE FACTOR

The filter function for the optical filter is defined as the ratio between the output power and input power. Assuming moderate efficiencies for the phase modulators, SLMs, and pinhole, $\eta^{\mathrm{A}} = 95\%$ and $\eta^{\mathrm{hole}} = 95\%$, we have $\gamma^{\mathrm{A}} \simeq 0.1\kappa$ and $\gamma_j^{\mathrm{hole}} \simeq 0.1\kappa e^{-|j|}$. With a typical value of 10MHz for $\kappa$, we calculate the filter function in the presence of imperfections discussed in section II, and plot the results in Fig. 6 in the main text. The calculation shows that, for a filter with a stop-band width of $4\kappa \simeq 40$MHz, a high skirt slope of $20dB/2$MHz can be obtained, leading to a shape factor of 0.85.


[1] Hernández, G. *Fabry-perot interferometers* (Cambridge University Press, Cambridge, 1986).

[2] Walls, D. F. and Milburn, G. J. *Quantum optics* (Springer-Verlag, Berlin, 2008).

[3] Yanik, M. F. and Fan, S. Stopping light all optically. *Phys. Rev. Lett.* **92,** 083901 (2004).

[4] Nagorny, B., Elsässer, T. and Hemmerich, A. Collective atomic motion in an optical lattice formed inside a high finesse cavity. *Phys. Rev. Lett.* **91,** 153003 (2003).

[5] Leidinger, M., Buse, K. and Breunig, I. Highly sensitive absorption measurements in lithium niobate using whispering gallery resonators. *Proc. SPIE* **9347,** 93471D (2015).

[6] Oemrawsingh, S. S. R., *et al.* Experimental demonstration of fractional orbital angular momentum entanglement of two photons. *Phys. Rev. Lett.* **95,** 240501 (2005).

[7] Marrucci, L., *et al.* Spin-to-orbital conversion of the angular momentum of light and its classical and quantum applications. *J. Opt.* **13,** 064001 (2011).

[8] Raut, H. K., Ganesh, V. A., Nair, A. S. and Ramakrishna, S. Anti-reflective coatings: A critical, in-depth review. *Energy Environ. Sci.* **4,** 3779–3804 (2011).

[9] Collins, S. A. Lens-system diffraction integral written in terms of matrix optics. *J. Opt. Soc. Am.* **60,** 1168–1177 (1970).

[10] Simon, C., *et al.* Quantum memories. *The Eur. Phys. J. D* **58,** 1–22 (2010).
